# Supplementary material for: VIGMA: An Open-Access Framework for Visual Gait and Motion Analytics
Source: arXiv:2504.17960 source file (2025-04-28)
Supplement: Supplementary file 1 [file appendix.tex]

\begin{table*}[t]
\caption{Requirement analysis from the survey questionnaire. We filtered the responses, focusing only on those that received at least 30\% of the votes (7 out of 23 participants), and used them to extract the relevant requirements for data processing, and data analysis and visualization tasks. Alongside the usage of computational notebooks, data processing requirements are subdivided into two groups namely: data standardization, and data management.}
\begin{tabular}{l|l|l}
\textbf{Survey Question (Q)}                                                                        & \textbf{Responses}                                                                                                                                                                                                                                                                                                                                                                                                           & \textbf{Requirements}                                                                                                                                                                                                                                                                                            \\\hline
\begin{tabular}[c]{@{}l@{}}Q1: What target population do \\ you collect data from?\end{tabular}   & \begin{tabular}[c]{@{}l@{}}• Healthy older adults (68.2\%)\\ • Stroke patients (54.5\%)\\ • Cognitive impaired patients (36.4\%)\\ • Healthy young adults (31.8\%)\end{tabular}                                                                                                                                                                                                                                          & \begin{tabular}[c]{@{}l@{}}\underline{Data management:} \\• Organized access to patient data.\end{tabular}                                                                                                                                                                                                                                                                         \\\hline
\begin{tabular}[c]{@{}l@{}}Q2: What is the primary goal of \\ your data collection?\end{tabular}  & \begin{tabular}[c]{@{}l@{}}• Understand biomechanics of gait (65.2\%).\\• Develop rehabilitation strategies (60.9\%).\\ • Compare gait features between \\trials/patients (52.2\%).\\• Predict future injury or fall risk (47.8\%).\\ • Monitoring disease progression over \\time (39.1\%).\\• Finding gait anomalies in a trial (30.4\%).\end{tabular}                                                              & \begin{tabular}[c]{@{}l@{}} \underline{Data analysis \& visualization:} \\• Analyze disease progression.\\ • Analyze group comparison.\\ • Analyze anomalies. \\ \\ \underline{Data standardization:} \\ • Extract fall risk using gait features.\\ \end{tabular}             \\\hline
\begin{tabular}[c]{@{}l@{}}Q3: What type of gait data do \\ you typically work with?\end{tabular} & \begin{tabular}[c]{@{}l@{}}• Spatiotemporal parameters (85\%).\\ • 3D marker trajectories (45\%).\\ • Ground reaction forces (40\%).\\ • Electromyography (40\%).\\ • Joint segment angles (35\%).\end{tabular}                                                                                                                                                                                                        & \begin{tabular}[c]{@{}l@{}} \underline{Data analysis \& visualization:} \\ • Analyze multivariate characteristics.\end{tabular}                                                                                                                                                                                                                                                          \\\hline
\begin{tabular}[c]{@{}l@{}}Q4: What are the formats of \\ data you collect?\end{tabular}          & \begin{tabular}[c]{@{}l@{}}• CSV (73.7\%).\\ • MAT (42.1\%).\\ • DAT (31.6\%).\\ • TXT (31.6\%).\end{tabular}                                                                                                                                                                                                                                                                                                            & \begin{tabular}[c]{@{}l@{}} \underline{Data standardization:} \\ •  Compatibility with multiple data formats.\end{tabular}                                                                                                                                                                                                                                                                     \\\hline
\begin{tabular}[c]{@{}l@{}}Q5: What data processing tasks\\  do you perform?\end{tabular}         & \begin{tabular}[c]{@{}l@{}} • Extract spatiotemporal features (e.g., stride \\length) (70\%)\\ • Mark step times in trial data (65\%)\\ • Predict step times from trial data (55\%)\\ • Normalize trials to gait cycle (50\%)\\ • Harmonize data formats (40\%)\\ • Extract joint angles from marker trajectories (30\%)\\ • Filter noise from trial (30\%)\\ • Predict missing values in trial (30\%)\end{tabular} & \begin{tabular}[c]{@{}l@{}}\underline{Data standardization}: \\  • Extract joint angles.\\ • Extract step times.\\• Extract spatiotemporal features. \\ • Fills missing values in trial. \\ • Filter noise from trial. \\ • Normalize trial by gait cycles.\end{tabular} \\\hline
\begin{tabular}[c]{@{}l@{}}Q6: What data analysis related\\  tasks do you perform?\end{tabular}   & \begin{tabular}[c]{@{}l@{}}• Exploring statistical measure (e.g., mean, \\median) (62.5\%)\\ • Analyzing patient data by groups (e.g., stroke \\patients) (50\%)\\ • Explore data for both single or multiple number of \\ patients/trials (43.8\%)\\ • Explore artifacts or outliers in the data (43.8\%)\end{tabular}                                                                                                          & \begin{tabular}[c]{@{}l@{}} \underline{Data analysis \& visualization:} \\ • Analyze statistical measures.\\ • Analyze anomalies \\ \\ \underline{Data management:} \\ • Organized access to patient data.\end{tabular}                                                                                                                                                                      \\\hline
\begin{tabular}[c]{@{}l@{}}Open-ended discussions\end{tabular}   & \begin{tabular}[c]{@{}l@{}}• Requirement of Live Scripts in MATLAB or Jupyter\\in Python for data processing tasks.\\ • Less code-intensive approach for data processing tasks.\\• Need to see numeric values alongside visualizations.\\ • Need to highlight specific data in visualizations.\\ • Highlighting data in one visualization should update\\corresponding data in other visualizations.\end{tabular}                                                                                                          & \begin{tabular}[c]{@{}l@{}} \underline{Data management:} \\ • Access to raw video. \\ \\ \underline{Data processing:} \\ • Computational notebooks.\\ \\ \underline{Data analysis \& visualization:} \\• Interactive analysis.\end{tabular}

% Require Live Scripts in MATLAB or Jupyter in Python for data processing tasks.
% Need to see numeric values alongside visualizations.
% Want to highlight data points in visualizations.
% Highlighting data in one visualization should automatically update corresponding data in other visualizations.

\end{tabular}
\label{table:survey}
\end{table*}

\clearpage

\begin{figure*}[t]
  \centering
  \includegraphics[width=\linewidth]{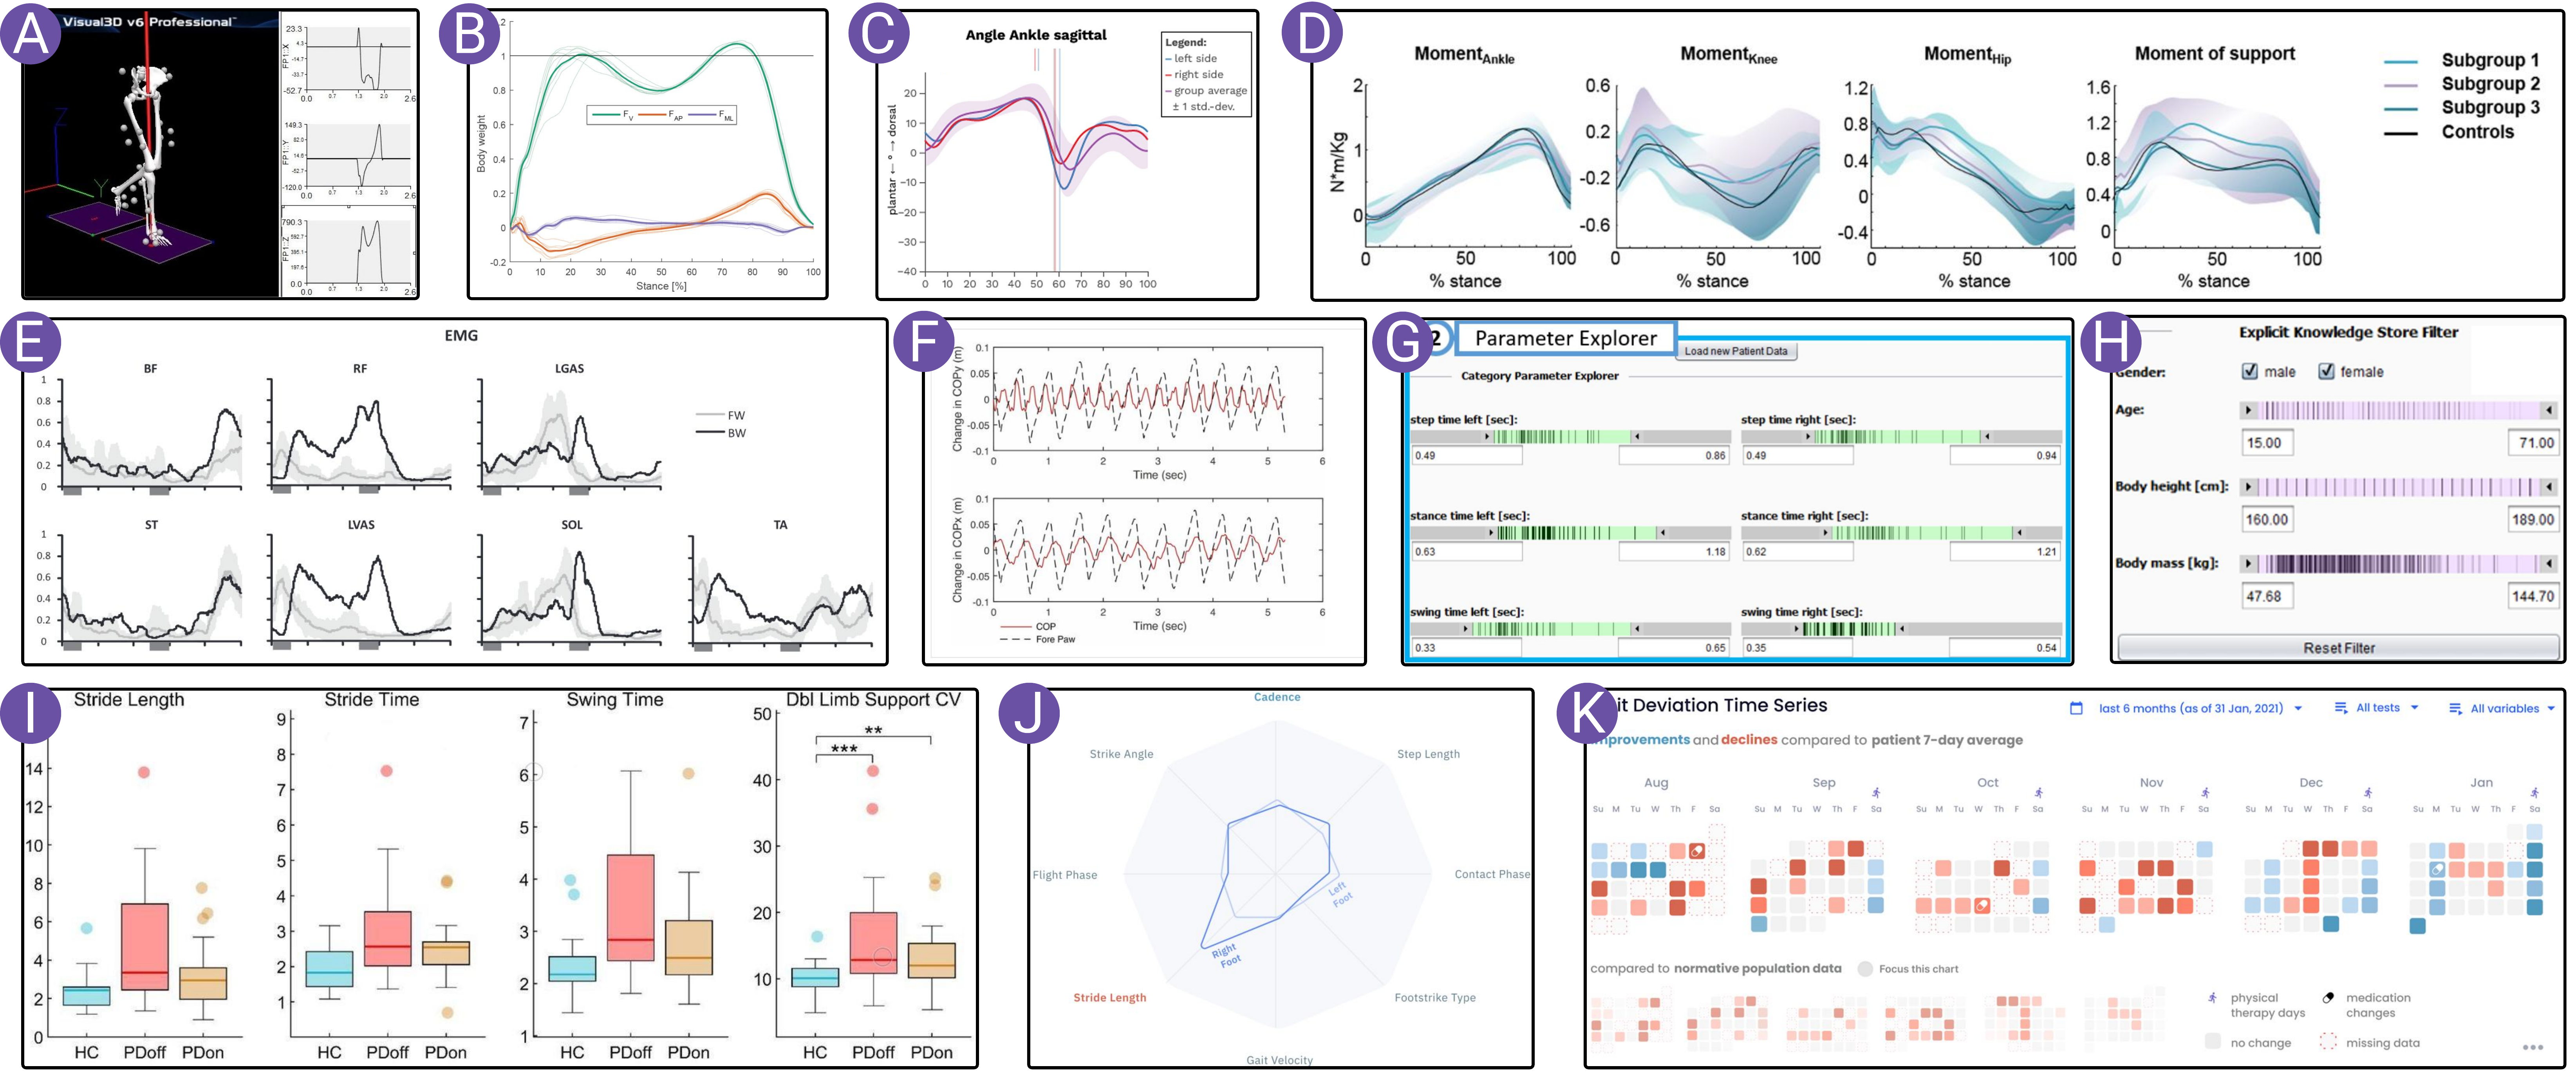}
  \caption{Visualizations curated from existing literature and gait analysis tools shown to the participants as part of the survey questionnaire. Participants evaluated the visualizations in terms of both \textbf{usability} and \textbf{understandability} and provided additional comments.}
  \label{fig:survey_vis}
\end{figure*}

\begin{table*}[h]
\centering
\caption{
Evaluation of visualizations A to K presented in Fig. \ref{fig:survey_vis} to 23 survey participants. Each visualization was categorized by its target attributes and visualization tasks. Participants scored each visualization in terms of usability and understandability on a scale of 1 to 10. The two different scores were combined to determine the mean score for each visualization.
}
\begin{tabular}{l|l|l|l|l|l}
\textbf{\#}      & \textbf{Visualization}      & \textbf{Target attributes}                                                                                           & \textbf{Visualization task}                                                    & \textbf{Source}                           & \begin{tabular}[c]{@{}l@{}}\textbf{Mean user score}\\(out of 10)\end{tabular}                                                           \\\hline

A                & Line plot                   & \begin{tabular}[c]{@{}l@{}}3D motion\end{tabular}                                             & • Display values                                                               & Visual3D~\cite{visual3d}                  & 7.2   \\\hline

B                & Line plot                   & \begin{tabular}[c]{@{}l@{}}Ground reaction forces.\\ • vertical (Fv)\\ • anterior-posterior (Fap)\\ • medial-lateral (Fml)\end{tabular} & \begin{tabular}[c]{@{}l@{}}• Display values\\ • Obtain data range\end{tabular} & KavaGait~\cite{wagner2018kavagait}        & 7.3   \\\hline

C                & Line plot                   & \begin{tabular}[c]{@{}l@{}}Joint angle\\ • sagittal ankle\end{tabular}                                               & \begin{tabular}[c]{@{}l@{}}• Display values\\ • Obtain data range\end{tabular} & gaitXplorer~\cite{rind2022trustworthy}    & 7.0   \\\hline

D                & Line plot                   & \begin{tabular}[c]{@{}l@{}}Joint moments. E.g.,\\ • knee\\ • hip\end{tabular}                                        & \begin{tabular}[c]{@{}l@{}}• Display values\\ • Obtain data range\end{tabular} & Serrao et al.~\cite{serrao2016gait}       & 6.5   \\\hline

E                & Line plot                   & \begin{tabular}[c]{@{}l@{}}Electromyography. E.g.,\\ • biceps femoris (BF)\\ • semitendinosus (ST)\end{tabular}      & \begin{tabular}[c]{@{}l@{}}• Display values\\ • Make comparisons\end{tabular}  & Jansen et al.~\cite{jansen2012similar}    & 6.9   \\\hline

F                & Line plot                   & Center of pressure                                                                                                   & \begin{tabular}[c]{@{}l@{}}• Display values\\ • Make comparisons\end{tabular}  & Blau et al.~\cite{blau2017quantifying}    & 6.7   \\\hline

G                & Strip plot                  & \begin{tabular}[c]{@{}l@{}}Spatiotemporal parameters. E.g.,\\ • stride length\\ • cadence\\ • swing time\end{tabular}                                                    & • Describe distribution                                                        & KavaGait~\cite{wagner2018kavagait}        & 6.7   \\\hline

H                & Strip plot                  & \begin{tabular}[c]{@{}l@{}}Patient demographics. E.g.,\\ • age\\ • gender\end{tabular}                               & • Describe distribution                                                        & KavaGait~\cite{wagner2018kavagait}        & 6.5   \\\hline

I                & Box plot                    & \begin{tabular}[c]{@{}l@{}}Spatiotemporal parameters\end{tabular}                                                    & \begin{tabular}[c]{@{}l@{}}• Describe distribution   \\ • Make comparisons\end{tabular}                                                        & Lopez et al.~\cite{troisi2021synthetic}   & 7.1   \\\hline

J                & Radar plot                  & \begin{tabular}[c]{@{}l@{}}Spatiotemporal parameters\end{tabular}& \begin{tabular}[c]{@{}l@{}}• Display values\\ • Make comparisons\end{tabular}  & Seals et al.~\cite{seals2022they}         & 7.2   \\\hline

K                & Calendar plot               & \begin{tabular}[c]{@{}l@{}}Spatiotemporal parameters\end{tabular}                                                    & \begin{tabular}[c]{@{}l@{}}• Make comparisons\end{tabular}                     & Seals et al.~\cite{seals2022they}         & 6.3

\end{tabular}
\label{table:survey_images}
\end{table*}

% \begin{figure*}[t]
%   \centering
%   \includegraphics[width=\linewidth]{}
%   \caption{Distribution of \textbf{usefulness} and \textbf{understandability} scores from the 23 survey participants. Overall, the participants scored the visualizations higher in terms of usefulness but lower in terms of understandibility. Red boxes around the charts shows visualizations where most participants scored the visualization 5 on a scale of 5, but at the same time black boxes show that for the same visualizations in terms of understandability most participants scored it 1 on a scale of 5.}
%   \label{fig:survey_dist}
% \end{figure*}

% \begin{figure}[h]
%   \centering
%   \includegraphics[width=\linewidth]{}
%   \caption{Distribution of understandability scores for visualizations grouped by participant demographics. For certain visualizations (D, F, G) highlighted in blue boxes show that students score the visualization overall higher than the other groups whereas in other cases (H, I, K) faculty scored the visualizations overall higher than the other groups.}
%   \label{fig:understandability_dist}
% \end{figure}

% \

\begin{figure*}[t]
  \centering
  \includegraphics[width=\linewidth]{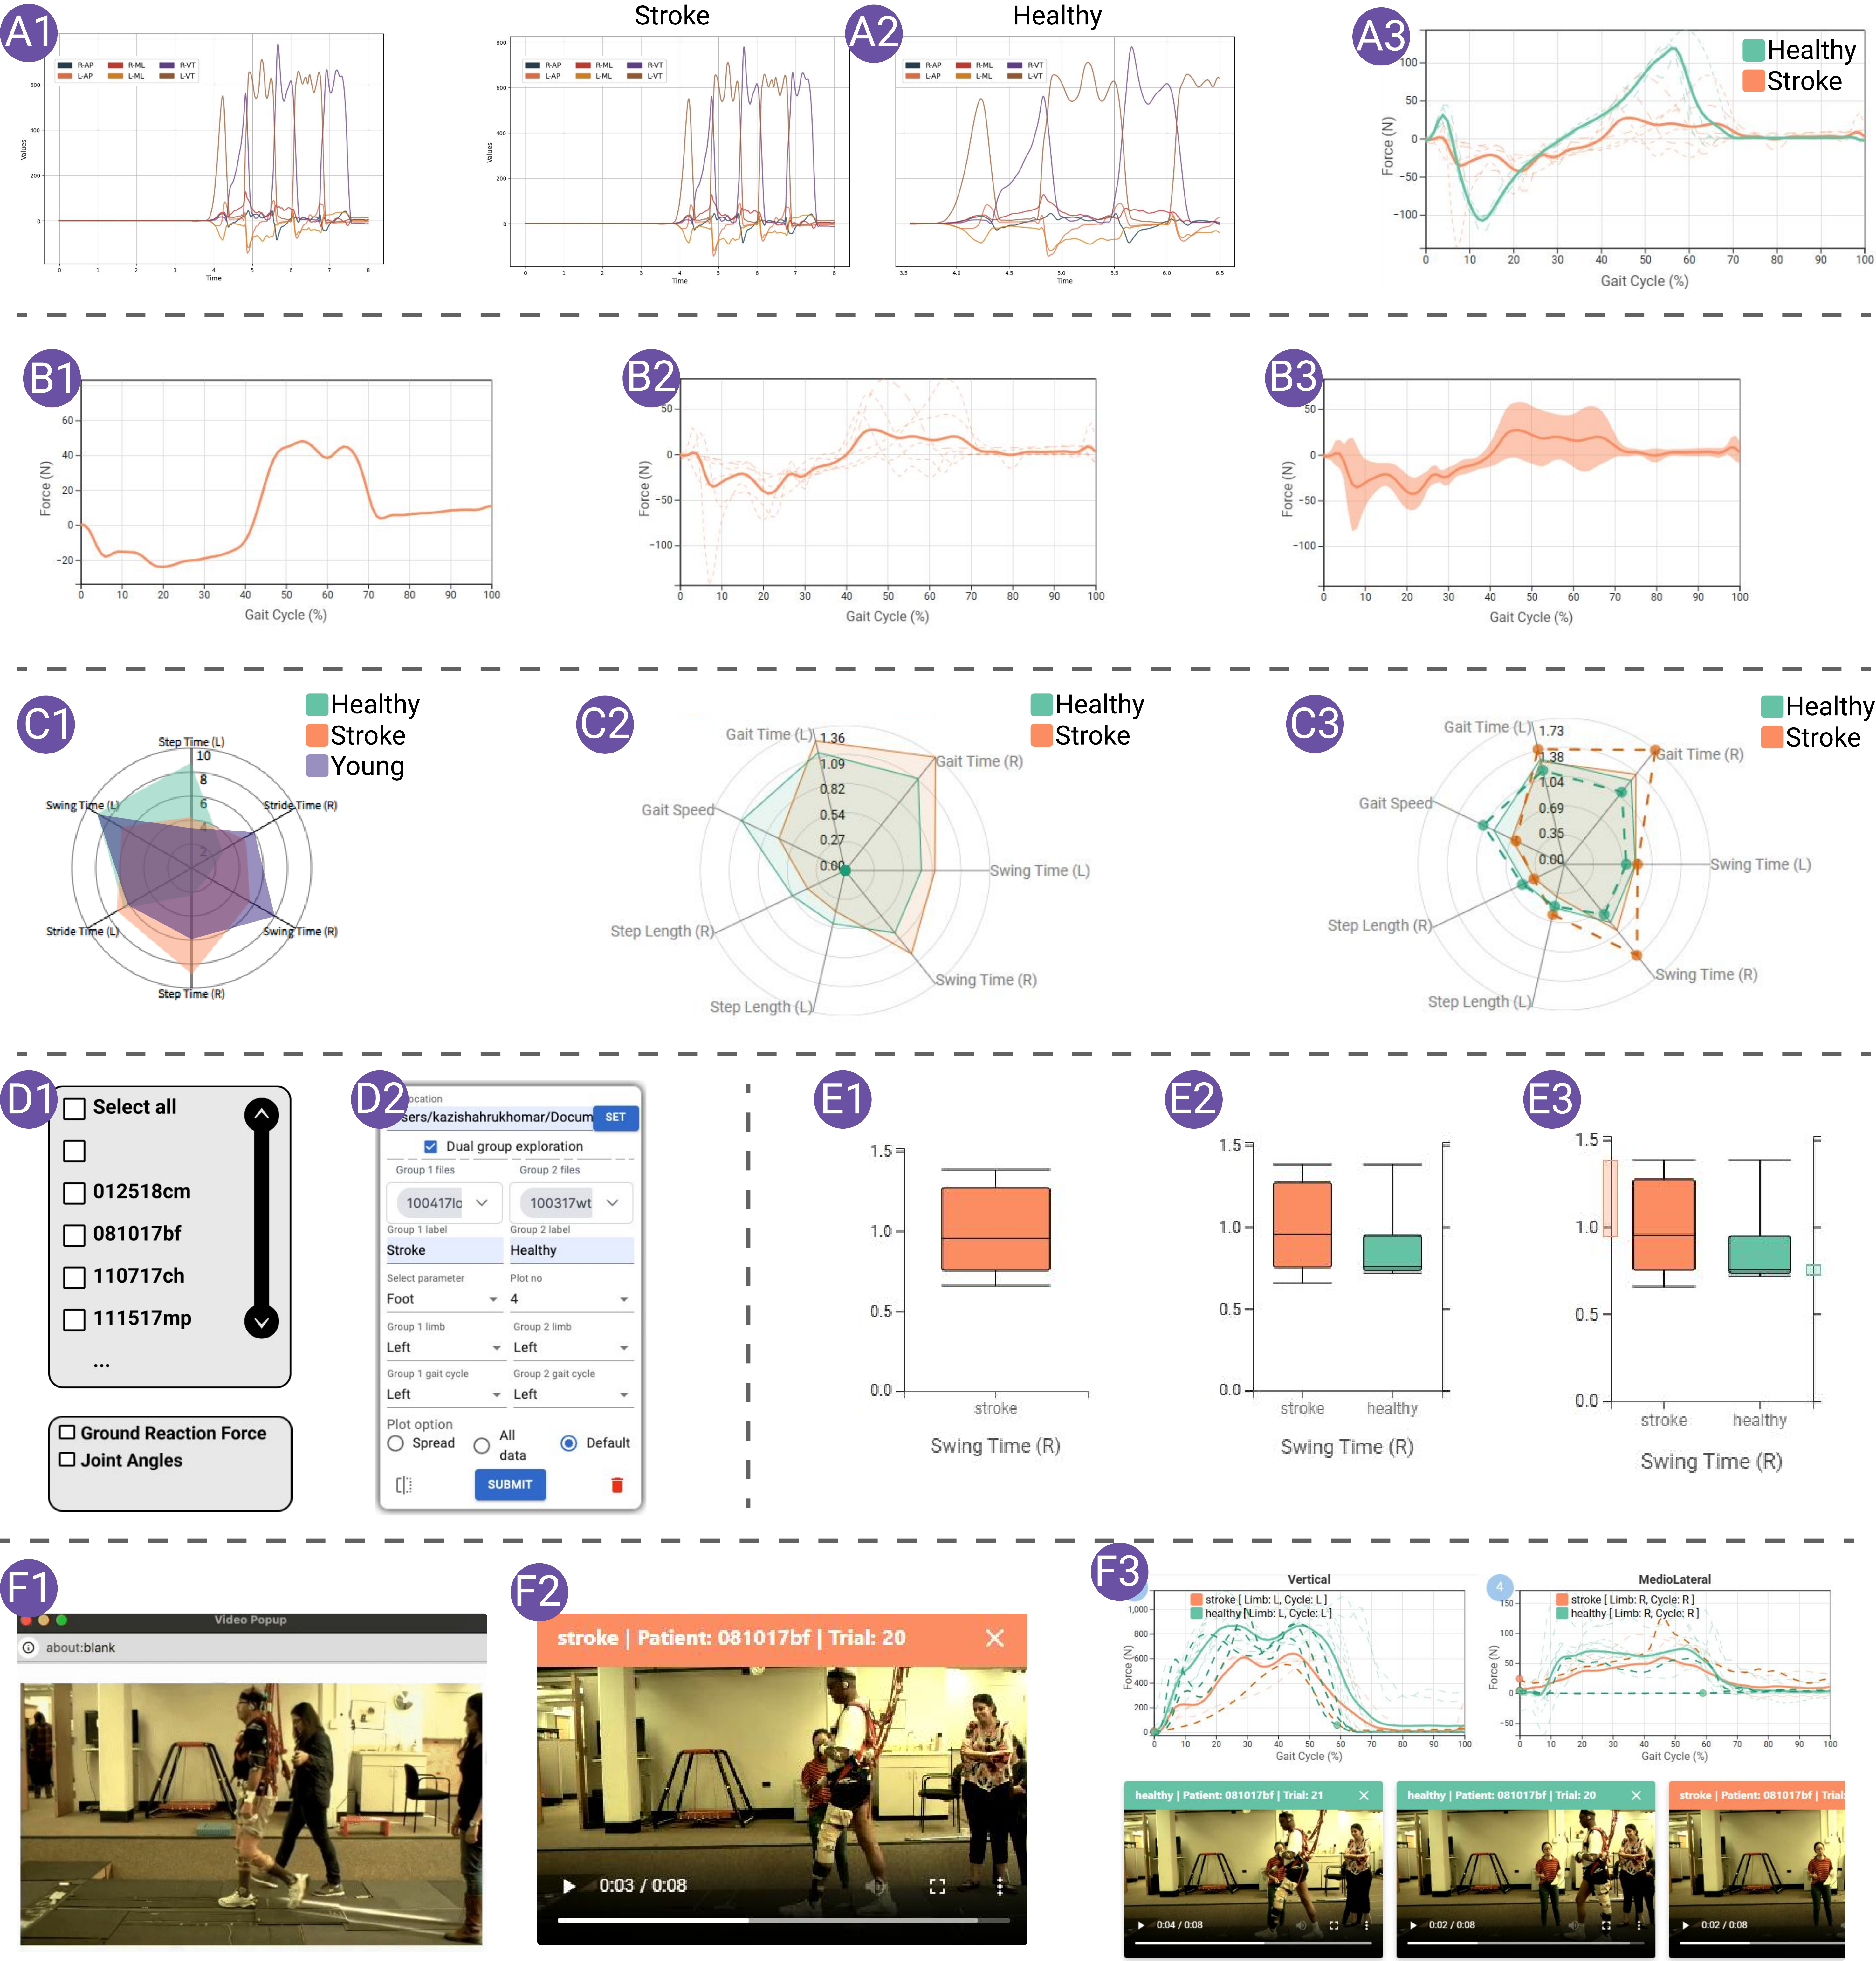}
  \caption{Alternative design choices in iterative development with expert feedback. For time-series visualization, we initially used (A1) a single chart displaying multiple attributes and (A2) side-by-side panels for group comparisons. Based on expert feedback and iterative discussions, we later transitioned to (A3) one attribute per panel, with two ensembles juxtaposed within the panel for comparison. Additionally, we moved from (B1) displaying only the mean of an attribute to providing options for (B2) showing all trials with the mean line and (B3) displaying the mean with confidence intervals. For spatiotemporal summaries, we transitioned from radar charts (C1) for more than three groups to (C2) only two groups and added option for (C3) highlighted trials. The control panel evolved from (D1) an initial rough layout to (D2) a cohesive design integrating all parameter options with hierarchical data management in one single place. Visualization of distribution progressed from (E1) a single box plot to (E2) dual box plots for group comparisons and (E3) interactive filtering via axis brushing. Video integration shifted from (F1) popups to (F2) video cards with patient info and video speed options, and finally to (F3) a scrollable video exploration view within the interface instead of popups.
  % Design of alternate interactions during development with feedback from the gait researchers. In the spatiotemporal summary view, we added \lower0.2em\hbox{\includesvg[width=1em]{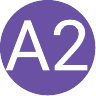}} dashed lines to highlight filtered trials within group ensembles, and we removed \lower0.2em\hbox{\includesvg[width=1em]{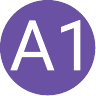}} the option to add trials separately in this view, merging it into the control panel. The control panel was redesigned several times. Instead of \lower0.2em\hbox{\includesvg[width=1em]{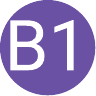}} selecting only patients, users can now \lower0.2em\hbox{\includesvg[width=1em]{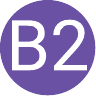}} select individual trials and configure various parameters for each group of ensembles. In the time series ensemble view, we initially showed \lower0.2em\hbox{\includesvg[width=1em]{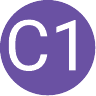}} all parameters in one view, but it was too cluttered, and the use of too many colors made it confusing. We redesigned this view so users can focus on one parameter's ensemble at a time, with options to view either \lower0.2em\hbox{\includesvg[width=1em]{icons/c2.svg}} the confidence intervals for each group or \lower0.2em\hbox{\includesvg[width=1em]{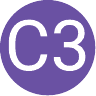}} individual trials, including options to highlight filtered trials.
  }
  \label{fig:interactions}
\end{figure*}

% All variables Ensemble mean -> One variable ensemble mean -> All trials along with ensemble mean -> Ensemble mean with CI

% Side by side comparison and focusing on all variables!! Comparison in a single chart with one variable with multiple panels for multiple variables!!

% Radar -> More than two ensembles -> Two ensembles 

% Single box plot -> Dual box plot

% Video popups -> Integrated in the interface -> Synchronized animated transition with time-series ensemble views!!
